# Supplementary material for: Enhancement of quantum heat engine by encircling a Liouvillian exceptional point
Source: arXiv:2302.13450 source file (2023-02-27)
Supplement: Supplementary file 1 [file supplementaryV4.pdf]

# Supplementary Materials for "Enhancement of quantum heat engine by encircling a Liouvillian exceptional point"

J.-T. Bu, J.-Q. Zhang, G.-Y. Ding, J.-C. Li, J.-W. Zhang, B. Wang, W.-Q. Ding, W.-F.. Yuan, L. Chen, S. K. Özdemir, F. Zhou, H. Jing, and M. Feng

# Supplementary Material for "Enhancement of quantum heat engine by encircling a Liouvillian exceptional point"

J.-T. Bu, J.-Q. Zhang, G.-Y. Ding, J.-C. Li, J.-W. Zhang, B. Wang, W.-Q. Ding, W.-F.. Yuan, L. Chen, S. K. Özdemir, F. Zhou, H. Jing, and M. Feng

## S1. I. EFFECTIVE HAMILTONIAN AND ITS DECAY RATE

The Hamiltonian describing the three-level single trapped ion in our experiment is given by,

$$H_s = \omega_e |e\rangle\langle e| + \omega_p |p\rangle\langle p| + \tfrac{\Omega}{2}(|e\rangle\langle g| e^{-i\omega_l t} + |g\rangle\langle e| e^{i\omega_l t}) + \tfrac{\Omega_p}{2}(|e\rangle\langle p| e^{-i\omega_d t} + |p\rangle\langle e| e^{i\omega_d t}), \tag{S1}$$

where $\omega_p$ and $\omega_e$ are, respectively, the energies of the levels $|p\rangle$ and $|e\rangle$ with respect to the ground level $|g\rangle$, and $\omega_l$ and $\omega_d$ are, respectively, the frequencies of the lasers coupling $|g\rangle$ to $|e\rangle$ and $|e\rangle$ to $|p\rangle$. $\Omega$ and $\Omega_p$ are, respectively, the coupling strengths for transitions $|g\rangle \longleftrightarrow |e\rangle$ and $|e\rangle \longleftrightarrow |p\rangle$.

This Hamiltonian $H_s$ follows the Schrödinger equation (in units of $\hbar = 1$)

$$\frac{d}{dt}|\psi\rangle_s = -iH_s|\psi\rangle_s, \tag{S2}$$

where $H_s = H_0 + H_1$ with $H_0$ being the time-independent part of the Hamiltonian.

Defining $|\psi\rangle_s = U_I|\psi\rangle_I$ with $U_I = e^{-iH_0 t}$, we rewrite the Schrödinger equation (S2) as

$$U_I^\dagger U_I \frac{d}{dt}|\psi\rangle_I = -i(U_I^\dagger H_s U_I - iU_I^\dagger \frac{dU_I}{dt})|\psi\rangle_I = -iH_I|\psi\rangle_I, \tag{S3}$$

leading to the interaction Hamiltonian $H_I$ as below,

$$H_I = U_I^\dagger H_s U_I - iU_I^\dagger \tfrac{dU_I}{dt} = U_I^\dagger H_s U_I - H_0. \tag{S4}$$

Defining $H_0 = \omega_l |e\rangle\langle e| + \omega_p |p\rangle\langle p|$ and using the Baker-Hausdorff formula

$$e^{iH_0 t} A e^{-iH_0 t} = A + it[H_0, A] + \frac{(it)^2}{2!}[H_0, [H_0, A]] + \cdots, \tag{S5}$$

we acquire the interaction Hamiltonian describing our experimental system as

$$H_I \;=\; \Delta |e\rangle\langle e| + \tfrac{\Omega}{2}(|e\rangle\langle g| + |g\rangle\langle e|) + \tfrac{\Omega_p}{2}(|e\rangle\langle p| + |p\rangle\langle e|), \tag{S6}$$

where $\Delta = \omega_e - \omega_l$ and $\omega_p = \omega_d + \omega_l$, $\omega_d = \omega_p - \omega_l = \omega_p - (\omega_e - \Delta) \simeq \omega_p - \omega_e$.

Using the effective operator formalism for open quantum systems as described in Ref. [S1], we obtain the following effective Hamiltonian $H_{\text{eff}}$

$$H_{\text{eff}} = -\tfrac{1}{2}V_-[H_{\text{NH}}^{-1} + (H_{\text{NH}}^{-1})^\dagger]V_+ = \Delta |e\rangle\langle e| + \tfrac{\Omega}{2}(|e\rangle\langle g| + |g\rangle\langle e|), \tag{S7}$$

where the non-Hermitian Hamiltonian $H_{\text{NH}}$ is given by $H_{\text{NH}} = -\frac{i}{2}(\gamma_e + \gamma_g)|p\rangle\langle p| = -\frac{i}{2}\gamma |p\rangle\langle p|$ with $\gamma_i$ corresponding to the decay rate from $|p\rangle$ to $|i\rangle$ and the perturbative excitations $V_+$ and de-excitations $V_-$ are defined as $V_+ = \frac{\Omega_p}{2}|p\rangle\langle e| + \frac{\Omega}{2}|e\rangle\langle g|$ and $V_- = \frac{\Omega_p}{2}|e\rangle\langle p| + \frac{\Omega}{2}|g\rangle\langle e|$.

Then we have the effective Lindblad operator as [S1]

$$L_{\text{eff}}^{e\to g} = i\sqrt{\gamma_g}\frac{\Omega_p}{\gamma}|g\rangle\langle e|, \tag{S8}$$

from which the effective decay rate $\gamma_{\rm eff}$ from the excited state $|e\rangle$ to the ground state $|g\rangle$ can be written as

$$\gamma_{\rm eff} = \frac{\gamma_g \Omega_p^2}{\gamma^2} = \frac{(\gamma - \gamma_e)\Omega_p^2}{\gamma^2} = (1 - \frac{\gamma_e}{\gamma})\frac{\Omega_p^2}{\gamma} \simeq \frac{\Omega_p^2}{\gamma}. \tag{S9}$$

The same result by an alternative method can be found in [S2]. We note that the expression for $H_{\rm eff}$ in Eq. (S7) and $\gamma_{\rm eff}$ appeared above are, respectively, the carrier-transition Hamiltonian and the effective decay rate employed in the main text.

## S2. II. LIOUVILLIAN EXCEPTIONAL POINTS

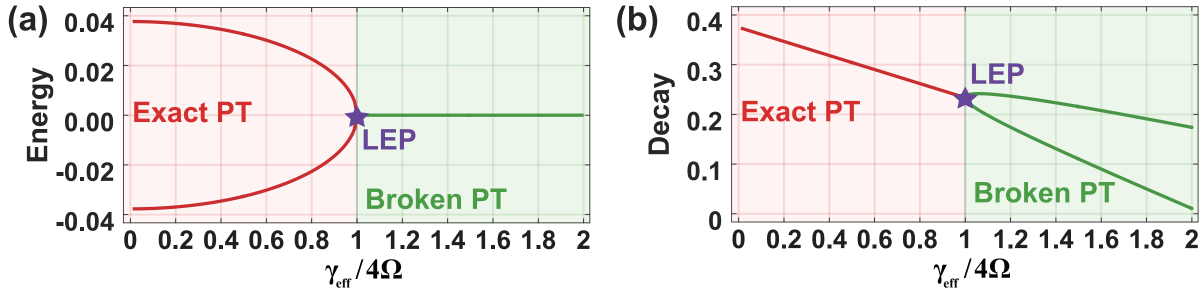


FIG. S1. (a) Eigenenergies Im$[\lambda_{3,4}]$ versus the decay rate $\gamma_{\rm eff}$. (b) Decay Re$[\lambda_{3,4}]$ versus the decay rate $\gamma_{\rm eff}$. Here we set $\Delta = 0$ and $\Omega = 1$.

The evolution of our system is described by the Lindblad master equation

$$\dot{\rho}(t) = -i[H_{\rm eff}, \rho] + \frac{\gamma_{\rm eff}}{2}(2\sigma_- \rho \sigma_+ - \sigma_+ \sigma_- \rho - \rho \sigma_+ \sigma_-) = \mathcal{L}\rho, \tag{S10}$$

where $\mathcal{L}$ is called Liouvillian superoperator and $\rho$ is the density operator of the system. From the Hamiltonian (S7) and the Lindblad master equation (S10), we write $\mathcal{L}$ as

$$\mathcal{L} = \begin{pmatrix} -\gamma_{\rm eff} & i\Omega/2 & -i\Omega/2 & 0 \\ i\Omega/2 & -(\gamma_{\rm eff}/2 + i\Delta) & 0 & -i\Omega/2 \\ -i\Omega/2 & 0 & -(\gamma_{\rm eff}/2 - i\Delta) & i\Omega/2 \\ \gamma_{\rm eff} & -i\Omega/2 & i\Omega/2 & 0 \end{pmatrix}. \tag{S11}$$

By setting $\Delta = 0$, we find the eigenvalues of $\mathcal{L}$ as $\lambda_1 = 0$, $\lambda_2 = -\gamma_{\rm eff}$, $\lambda_3 = \frac{1}{4}(-3\gamma_{\rm eff} - \sqrt{\gamma_{\rm eff}^2 - 16\Omega^2})$, and $\lambda_4 = \frac{1}{4}(-3\gamma_{\rm eff} + \sqrt{\gamma_{\rm eff}^2 - 16\Omega^2})$. Since these eigenvalues are related to the dissipation terms, their real parts indicate the decaying effects, while their imaginary parts define the eigenenergies [S3]. When $\gamma_{\rm eff} = 4\Omega$, $\lambda_3$ and $\lambda_4$ turn to be degenerate and a LEP appears at $\lambda_3 = \lambda_4 = -3\gamma_{\rm eff}/4$. As explained in the main text, for $\gamma_{\rm eff} > 4\Omega$, we have real $\lambda_3$ and $\lambda_4$ with the splitting $|\lambda_3 - \lambda_4| = 2\xi = \sqrt{\gamma_{\rm eff}^2 - 16\Omega^2})$. Thus, when $\gamma_{\rm eff} > 4\Omega$, the system is in the broken phase. In contrast, for $\gamma_{\rm eff} < 4\Omega$, $\lambda_3$ and $\lambda_4$ become complex conjugate pairs with a splitting of $2\xi$ in their imaginary parts, corresponding to the exact phase (see Fig. S1).

## S3. III. DYNAMICS OF QUANTUM HEAT ENGINE CYCLES

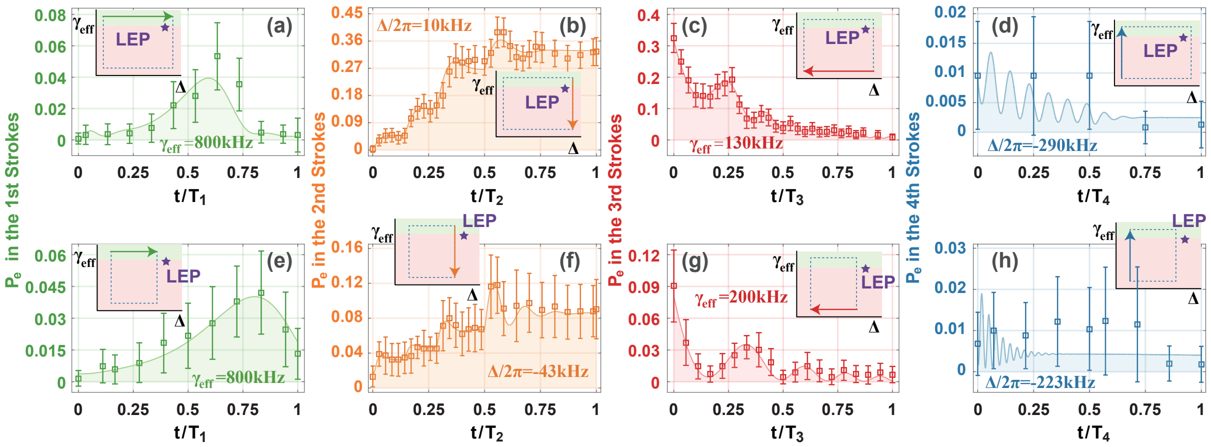

FIG. S2. Measured populations of the excited state in QHE cycles. (a), (b), (c) and (d) are for the first, second, third and fourth strokes, respectively, when encircling the LEP ($\Delta_{\rm min}/2\pi = -290$ kHz, $\gamma_{\rm max} = 800$ kHz, $\Delta_{\rm max}/2\pi = 10$ kHz, $\gamma_{\rm min} = 130$ kHz). The durations of the strokes in the cycle are $T_1 = 30$ $\mu$s, $T_2 = 140$ $\mu$s, $T_3 = 30$ $\mu$s, and $T_4 = 40$ $\mu$s, with $\Omega/2\pi$ fixed to be 29 kHz ; (e), (f), (g) and (h) represent the first, second, third and fourth strokes, respectively, during the loop that does not encircle the LEP ($\Delta_{\rm min}/2\pi = -223$ kHz, $\gamma_{\rm max} = 800$ kHz, $\Delta_{\rm max}/2\pi = -43$ kHz, $\gamma_{\rm min} = 200$ kHz). The strokes in the cycle take $T_1 = 18$ $\mu$s, $T_2 = 140$ $\mu$s, $T_3 = 18$ $\mu$s, and $T_4 = 140$ $\mu$s. Throughout the cycles, $\Omega/2\pi$ remains to be 29 kHz.

We execute the two cycles of the quantum heat engine (QHE) as designed in Fig. 1(b) of the main text by elaborately controlling the 854-nm laser (for tuning $\gamma_{\rm eff}$) and the 729-nm laser (for detuning $\Delta$).

We observe the dynamical process of the big QHE cycle encircling the LEP by monitoring the evolution of the population $P_2$, as shown in Fig. S2(a-d). We fix $\Omega/2\pi = 29$ kHz throughout the QHE cycle, and first execute the iso-decay compression process (Fig. S2(a) for $T_1 = 30$ $\mu$s) by increasing the detuning $\Delta$ from $\Delta_{\rm min} = -290 \times 2\pi$ kHz to $\Delta_{\rm max} = 10 \times 2\pi$ kHz while $\gamma_{\rm eff} = \gamma_{\rm max} = 800$ kHz remains unchanged. A hump is observed in the population $P_2$ due to Landau-Zener transition. Then we carry out the isochoric heating process (Fig. S2(b) for $T_2 = 140$ $\mu$s) by reducing the decay rate $\gamma_{\rm eff}$ from $\gamma_{\rm max} = 800$ kHz to $\gamma_{\rm min} = 130$ kHz while $\Delta = \Delta_{\rm max}$ is fixed. For simplicity, we divide the evolution time into four steps in the decrease of the decay rate, i.e., $T_{2-1} = 20$ $\mu$s, $\gamma_{\rm eff} \simeq 800$ kHz; $T_{2-2} = 20$ $\mu$s, $\gamma_{\rm eff} \simeq 577$ kHz; $T_{2-3} = 30$ $\mu$s, $\gamma_{\rm eff} \simeq 353$ kHz; and $T_{2-4} = 70$ $\mu$s, $\gamma_{\rm eff} \simeq 130$ kHz. During this process, we have observed the population increase in an oscillatory way, which might be due to the interplay between quantum coherence and the increasing decay. The next stroke is the iso-decay expansion (Fig. S2(c) for $T_3 = 30$ $\mu$s) with the detuning tuned from $\Delta_{\rm max}$ back to $\Delta_{\rm min}$ with the constant value of $\gamma_{\rm eff} = \gamma_{\rm min}$. We have observed the damped population oscillation from the second Landau-Zener transition, actually implying the Stückleberg phase effect. The final step is the isochoric cooling process (Fig. S2(d) for $T_4 = 40$ $\mu$s) with the decay rate $\gamma_{\rm eff}$ tuned from $\gamma_{\rm min} = 130$ kHz to $\gamma_{\rm max} = 800$ kHz when $\Delta = \Delta_{\rm min}$ is fixed. During this process, we divide the evolution time into two stages in the increase of the decay rate, i.e., $T_{4-1} = 20$ $\mu$s, $\gamma_{\rm eff} \simeq 130$ kHz and $T_{4-2} = 20$ $\mu$s, $\gamma_{\rm eff} \simeq 800$ kHz). We have observed that the population $P_2$ in this stroke is severely suppressed due to the large detuning, and the small population oscillation, as theoretically predicted, is hard to be observed experimentally. With the assistance of the large decay rate, our system returns to the initial steady state.

Similarly, the dynamical process of the small QHE cycle without enclosing the LEP is demonstrated in Fig. S2(e-h) by monitoring the varying population $P_2$ with $\Omega/2\pi = 29$ kHz fixed throughout the

cycle. Different from the case of the big QHE cycle, we set the parameters as $\Delta_{\rm min}/2\pi$ = -223 kHz, $\Delta_{\rm max}/2\pi = -43$ kHz, $\gamma_{\rm min} = 200$ kHz, $\gamma_{\rm max} = 800$ kHz, $T_1 = T_3 = 18\mu$s, and $T_2 = T_4 = 140\mu$s. Besides, we implement the fourth stroke with four steps as $T_{4-1} = 70\mu$s, $\gamma_{\rm eff} \simeq 130$ kHz; $T_{4-2} = 30\mu$s, $\gamma_{\rm eff} \simeq 353$ kHz; $T_{4-3} = 20\mu$s, $\gamma_{\rm eff} \simeq 577$ kHz; $T_{4-4} = 20\mu$s, $\gamma_{\rm eff} \simeq 800$ kHz.

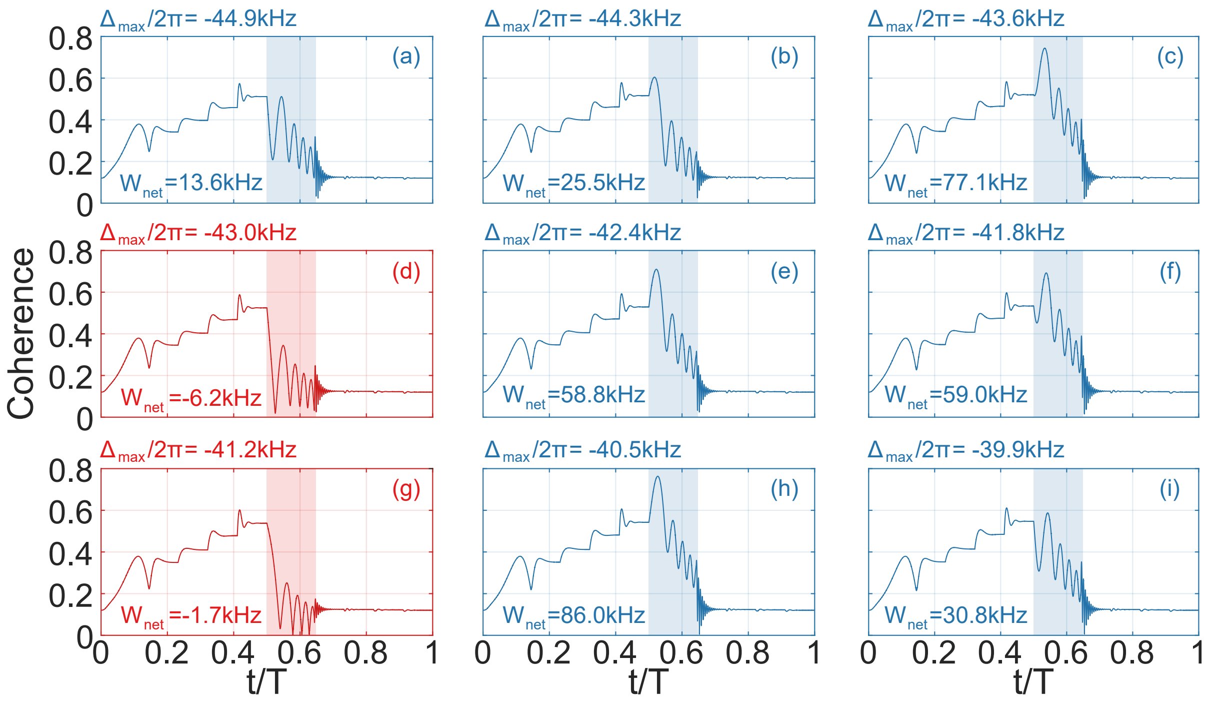


FIG. S3. Time evolution of coherence in small QHE cycles that do not encircle the LEP for different values of $\Delta_{\rm max}$. We set parameters as $\Delta_{\rm min}/2\pi = -223$ kHz, $\Delta_0/2\pi = -43$ kHz, $\gamma_{\rm max} = 800$ kHz, $\gamma_{\rm min} = 200$ kHz, $T = T_1 + T_2 + T_3 + T_4$, $T_1 = T_3 = \frac{\Delta_{\rm max}-\Delta_{\rm min}}{\Delta_0-\Delta_{\rm min}} \times 18$ $\mu$s, $T_2 = T_4 = 140$ $\mu$s, and $\Omega/2\pi = 29$ kHz.

## S4. IV. THERMODYNAMIC QUANTITIES

In this section, we discuss the definitions for the net work $W_{\rm net}$ and the efficiency $\eta$. For the QHE system based on a trapped ion, we define the internal energy of the spin heat engine as $U = {\rm tr}(\rho H)$ [S4], where $\rho$ and $H$ are the density matrix and Hamiltonian of the spin system, respectively. In our case, the Hamiltonian of the system is $H = \Delta \left|e\right\rangle\left\langle e\right|$, and the coupling strength $\Omega$, and the effective dissipation rate $\gamma_{\rm eff}$ are tuned to perform the QHE cycles, as elucidated in the main text.

While the conventional first law of thermodynamics is expressed as $dU = dW + dQ$, its counterpart in quantum thermodynamics is expressed as $dU = d({\rm tr}(\rho H)) = {\rm tr}(\rho dH) + {\rm tr}(H d\rho)$, where the work and heat are defined, respectively, as $dW = \rho dH$ and $dQ = H d\rho$ in the differential forms. Then the work $W_{\rm in} = -\sum_i \rho_i dH'_i = -\int_0^t \rho_i(t) dH'_i$ (for $dH'_i > 0$) describes the work performed by the baths to the system in the iso-decay compression, and $W_{\rm out} = -\sum_i \rho_i dH'_i = -\int_0^t \rho_i(t) dH'_i$ (for $dH'_i < 0$) denotes the work performed by the system on the baths in the iso-decay expansion. As such, the net work of the QHE

cycle can be written as

$$W_{\rm net} \;=\; W_{\rm in} + W_{\rm out} = -\sum_i \rho_i dH_i' = -\int_0^t \rho_i(t) dH_i', \tag{S12}$$

which is used to calculate the net work in the main text Fig. 2.

The efficiency is an important quantity for the performance of the QHE and it is given by

$$\eta \;=\; \frac{W_{\rm net}}{Q_{\rm in}}, \tag{S13}$$

where $Q_{\rm in} = \sum_i H_i d\rho_i' = \int_0^t H_i d\rho_i'$ (for $d\rho_i' > 0$) denotes the energy absorption from the baths in all the QHE cycles.

## S5. V. QUANTUM COHERENCE

We define the coherence as $C_{l_1}(\rho) = \sum_{i\neq j} |\rho_{i,j}|$ [S5], and evaluate the coherence involved in the two QHE cycles for different values of $\Delta_{\rm max}$ in Figs. S3 and S4, where the red and blue curves correspond to the cases with negative and positive net works, respectively.

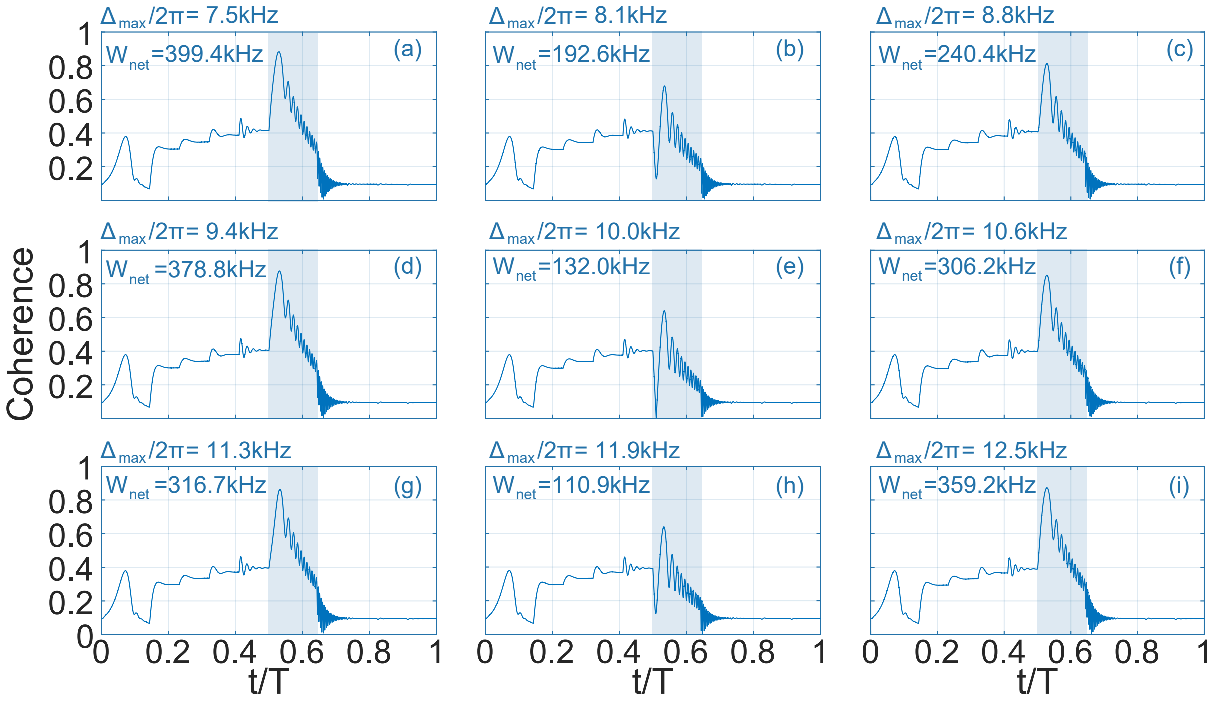


FIG. S4. Time evolution of coherence in big QHE cycles that encircle the LEP for different values of $\Delta_{\rm max}$. We set parameters as $\Delta_{\rm min}/2\pi = -290$ kHz, $\Delta_0/2\pi = 10$ kHz, $\gamma_{\rm max} = 800$ kHz, $\gamma_{\rm min} = 200$ kHz, $T = T_1 + T_2 + T_3 + T_4$, $T_1 = T_3 = \frac{\Delta_{\rm max}-\Delta_{\rm min}}{\Delta_0-\Delta_{\rm min}} \times 30$ $\mu$s, $T_2 = T_4 = 140$ $\mu$s, and $\Omega/2\pi = 29$ kHz.

As our QHE cycles are implemented in a closed way, we see in both the figures that values of coherence return their initial values at the end of the cycles. Moreover, in each panel, whether the net work is

negative or positive is relevant to the coherence variation in the shaded regions (corresponding to the third stroke). We find that the small mean values of the coherence within the shaded regions lead to the negative net work, which happen in some cases of the small QHE cycle. However, no such small value of coherence is found in the big QHE cycle, and thus the big QHE cycles produce definitely positive net work. We think that this is because the big QHE cycles experience complete Landau-Zener-Stückleberg interference, acquiring sufficient coherence from the driving laser field.

## S6. VI. LEP-ENHANCED EFFICIENCY

In this section, we carry out numerical simulation for the efficiency of the QHE cycles, corresponding to the net works demonstrated in the main text Fig. 3. In Fig. S5 we see the curves behaving similarly to those in the main text Fig. 3: the efficiency can be positive or negative if the LEP ($\Delta = 0$) is not encircled; while is definitely positive once the LEP is enclosed in the QHE cycle. In addition, the largest efficiency exists close to the LEP.

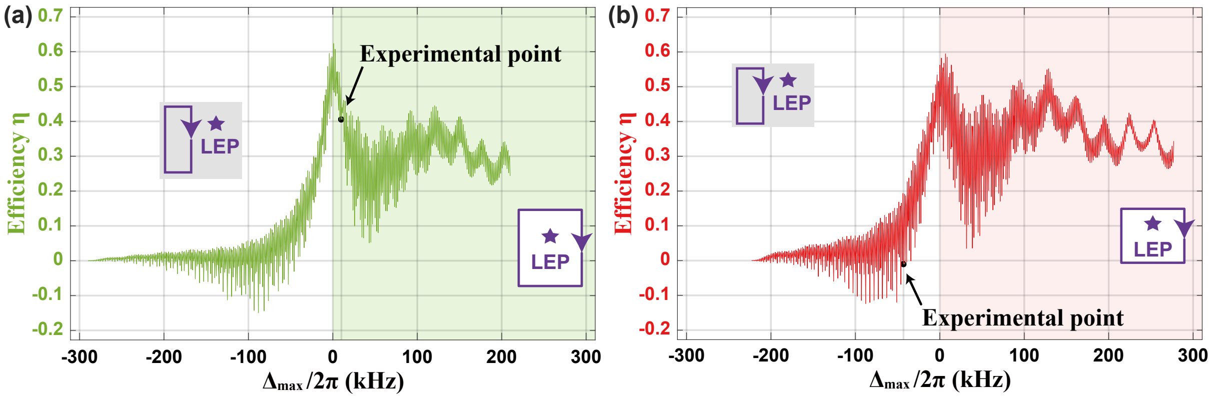


FIG. S5. Numerical results depicting the effect of $\Delta_{\max}$ on the efficiency of the QHE. (a) The situation covering the big cycle executed in the experiments, where the QHE cycle starts from the point A with $\Delta_{\min}/2\pi = -290$ kHz and $\gamma_{\max} = 800$ kHz, sweeping the frequency to $\Delta_{\max}/2\pi \leqslant 210$ kHz. So the point C is set with -289.9 kHz $\leqslant \Delta_{\max}/2\pi \leqslant 210$ kHz and $\gamma_{\min} = 130$ kHz. (b) The situation involving the small cycle executed in the experiments, where the QHE cycle starts from A with $\Delta_{\min}/2\pi = -223$ kHz and $\gamma_{\max} = 800$ kHz, sweeping the frequency to $\Delta_{\max}/2\pi \leqslant 277$ kHz. So the point C is set with -222.9 kHz $\leqslant \Delta_{\max}/2\pi \leqslant 277$ kHz and $\gamma_{\min} = 200$ kHz. In both the panels, the black dots indicate the maximal detuning reached in our experiment, and we consider 804 points as the values of the maximal detuning.

## S7. VII. THE QHE WITH NONLINEARLY VARYING ISO-DECAY PROCESSES

To further verify the positive net work relevant to the LEP, we numerically calculate the population $P_2$ and the net work $W_{\rm net}$ of the QHE cycles with nonlinear variation of the detuning in the first and third strokes. The results presented in Fig. S6 demonstrate the similar behaviors to in Fig. 2 of the main text, indicating that the non-adiabatic evolutions in the iso-decay processes can be controlled by whether linear or nonlinear variation of the detuning.

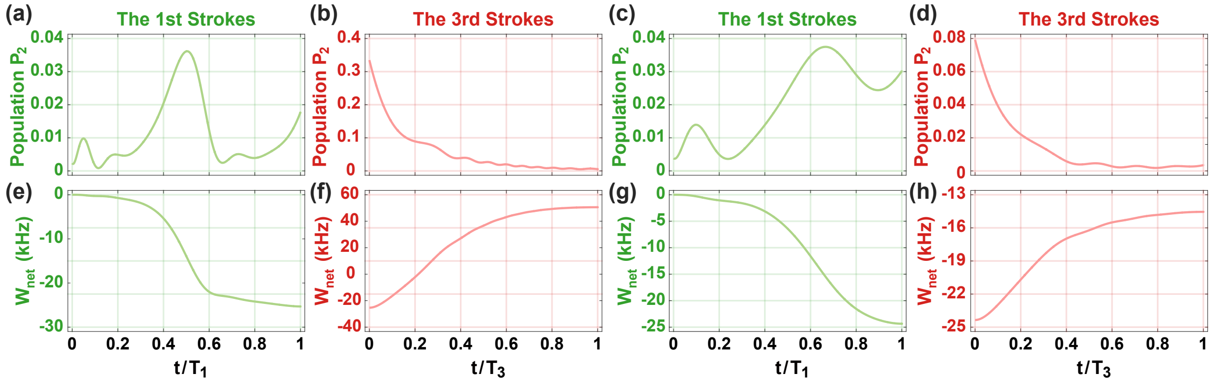


FIG. S6. Simulation of the population $P_2$ of the excited state in iso-decay strokes, where (a) and (b) are for the first and third strokes, respectively, in the case of encircling the LEP ($\Delta_{\min}/2\pi = -290$ kHz, $\Delta_{\max}/2\pi = 9.0$ kHz, $\gamma_{\min} = 130$ kHz, and $\gamma_{\max} = 800$ kHz). The time is set as $T_1 = T_3 = 29.9$ $\mu$s. (c) and (d) represent the first and third strokes, respectively, in the case of not encircling the LEP ($\Delta_{\min}/2\pi = -223$ kHz, $\Delta_{\max}/2\pi = -43.65$ kHz, $\gamma_{\min} = 200$ kHz, and $\gamma_{\max} = 800$ kHz). The time is $T_1 = T_3 = 17.9$ $\mu$s. (e, f, g, h) Net work corresponding to the panels (a, b, c, d), respectively. In all the panels, $\Omega/2\pi = 29$ kHz. We set $\Delta = \frac{\Delta_{\max}+\Delta_{\min}}{2} - \frac{\Delta_{\max}-\Delta_{\min}}{2}\cos(2\pi t/T_1)$ for the 1st stroke and $\Delta = \frac{\Delta_{\max}+\Delta_{\min}}{2} + \frac{\Delta_{\max}-\Delta_{\min}}{2}\cos(2\pi t/T_3)$ for the 3rd stroke.


[S1] Florentin Reiter and Anders S. S$\phi$rensen, "Effective operator formalism for open quantum systems", Phys. Rev. A. **85**, 032111 (2019).

[S2] J. W. Zhang, K. Rehan, M. Li, J. C. Li, L. Chen, S.-L. Su, L.-L. Yan, F. Zhou, and M. Feng, "Single-atom verification of the information-theoretical bound of irreversibility at the quantum level", Phys. Rev. Research **2**, 033082 (2020).

[S3] F. Minganti, A. Miranowicz, R. W. Chhajlany, and F. Nori, "Quantum exceptional points of non-Hermitian Hamiltonians and Liouvillians: The effects of quantum jumps", Phys. Rev. A **100** 062131 (2019).

[S4] H. T. Quan, Yu-xi Liu, C. P. Sun, and Franco Nori, "Quantum thermodynamic cycles and quantum heat engines", Phys. Rev. E. **76**, 031105 (2007).

[S5] T. Baumgratz, M. Cramer, and M. B. Plenio, "Quantifying Coherence", Phys. Rev. Lett. **113**, 140401 (2014).
